# Supplementary material for: Learning Representations for Counterfactual Inference
Source: arXiv:1605.03661 source file (2018-06-06)
Supplement: Supplementary file 1 [file appendix.tex]

\section{Linear discrepancy}
\label{app:lindisc}
We show that
$$
\disc(P,Q) = \|\mu_2(P) - \mu_2(Q)\|_2
$$

\section{Bounding $g_2$}
An alternate route for bounding $g_2$ is by assuming that the treatment effect is bounded in absolute value by $r$, i.e. for the unit $i$ we have $|y^F_i - y^{CF}_i| \leq r$. With a similar analysis to the case of $y^{CF}_i \in [-M, M]$, we have that
$$g_2(\Phi,v) = r + \frac{1}{n} \sum_{i=1}^n |\hat{y}_i^{CF}(\Phi,v) - y_i^F|.$$
In this alternate route, neglecting the constant terms, we end up with $$g(\Phi,v) = \frac{1}{n} \sum_{i=1}^{n}\left( |y^F_i - \hat{y}_i^F(\Phi,v) \, | + |y_i^F - \hat{y}_i^{CF}(\Phi,v) | \right).$$

\section{Evaluation metrics}
\label{app:eval}

\paragraph{Error in counterfactual outcome}
$$
\epsilon_{Y^{CF}} = \sqrt{\frac{1}{n} \sum_{i=1}^n
\left(\hat{Y}^{CF}_{x_i} - Y^{CF}_{x_i}\right)^2}
$$

\paragraph{Error in individual treatment effect}
$$
\epsilon_{ITE} = \sqrt{\frac{1}{n} \sum_{i=1}^n
\left(\frac{\hat{Y}^{CF}_{x_i} - Y^{F}_{x_i}}{1-2t_i} - \expect[Y^1_{x_i}-Y^0_{x_i}]\right)^2}
$$

\paragraph{Error in average treatment effect}
$$
\epsilon_{ATE} = \left| \frac{1}{n} \sum_{i=1}^n
\frac{\hat{Y}^{CF}_{x_i} - Y^{F}_{x_i}}{1-2t_i} - \frac{1}{n} \sum_{i=1}^n \expect[Y^1_{x_i}-Y^0_{x_i}] \right|
$$
\fxfatal{Currently we report the RMSE over experiments}

\paragraph{PEHE}
$$
PEHE = \sqrt{\frac{1}{n} \sum_{i=1}^n
\left(\hat{Y}^{1}_{x_i} - \hat{Y}^{0}_{x_i} - \expect[Y^1_{x_i}-Y^0_{x_i}]\right)^2}
$$
